# Supplementary material for: Superspin Glass Mediated Giant Spontaneous Exchange Bias in a Nanocomposite of BiFeO$_3$-Bi$_2$Fe$_4$O$_9$
Source: arXiv:1202.5898 source file (2013-04-01)
Supplement: Supplementary file 1 [file supplementary.pdf]

## The Supplementary Document

This supplementary document contains detailed results from high resolution powder x-ray diffraction (XRD), transmission electron microscopy (TEM), and magnetic measurements. They are organized as follows: first, we are showing the room temperature x-ray diffraction data refined by FullProf. The refinement yields the microstructural details such as (a) crystallite size, strain and (b) volume fraction of each phase as well as crystallographic details such as (a) lattice parameters, (ii) atom positions, (iii) bond length and angle etc. In Fig. 1 of this supplementary document, the Rietveld refined x-ray diffraction data are given. In Table-I we give the detailed results of the refinement. The average grain size for  $\text{BiFeO}_3$  phase is  $\sim 112$  nm whereas that for  $\text{Bi}_2\text{Fe}_4\text{O}_9$  phase is  $\sim 19$  nm in sample-A. In sample-B, the grain size for  $\text{BiFeO}_3$  and  $\text{Bi}_2\text{Fe}_4\text{O}_9$  phases turn out to be  $\sim 30$  nm and  $\sim 8$  nm, respectively. In sample-C, the average grain size for  $\text{BiFeO}_3$  phase is  $\sim 12$  nm. The volume fraction of  $\text{Bi}_2\text{Fe}_4\text{O}_9$  phase in sample-A is  $\sim 6\%$  whereas for sample-B and C they are  $\geq 10\%$ , and  $\leq 3\%$ .

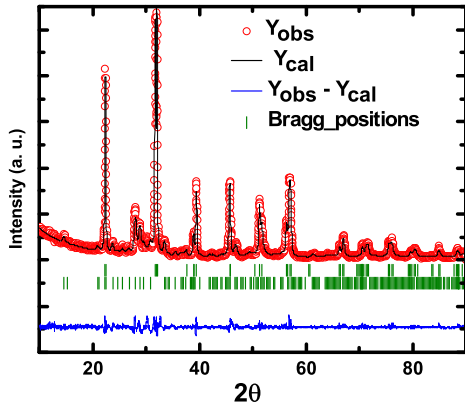

FIG. 1. (color online) The room temperature x-ray diffraction pattern of the nanocomposite. The pattern has been refined by FullProf.

In Fig. 2, we show the bright and dark field (BF/DF) TEM images of the sample-A. A comparison of the BF/DF images shows an intimate mixing of the two phases which has given rise to a high interface density in sample-A. The selected area electron diffraction (SAED) patterns as well as high resolution TEM (HRTEM) images have also been recorded. The particles are single crystalline. The spots in the SAED images have been indexed by taking into consideration the distance between the lattice planes  $d$ , angle between the planes  $\phi$ , as well as the Weiss zone law. Detailed study of the SAED pat-

terns helped in identifying the zone axes for both the  $\text{BiFeO}_3$  and  $\text{Bi}_2\text{Fe}_4\text{O}_9$  particles. The tilt between the crystals turn out to be  $\sim 19^\circ$  for a test case. The convergent beam electron diffraction (CBED) patterns have also been recorded (data not shown) at a few places of the composite. The diffraction spots have been indexed accurately using the method described above. However, a detailed mapping of the variation in tilt across the entire matrix of the nanocomposite could not be completed due to lack of satisfactory images from different regions of the nanocomposite. The scale of mixing of the phases and the resolution at which the images could be captured differed by a large extent at many places.

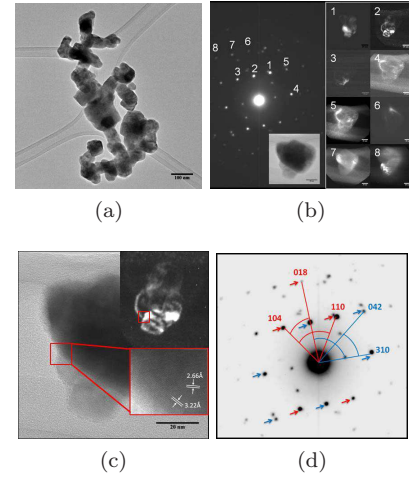

FIG. 2. (color online) (a) A representative bright-field TEM image of the nanocomposite; (b) the SAED patterns showing diffraction spots from both the phases; the dark-field images (marked by numbers) in the side panel shows the regions of the particles corresponding to the diffraction spots; inset shows the bright-field image of the region; the bright-field/dark-field images together with electron diffraction patterns from the regions show the dispersion of the phases and the interfaces in the nanocomposite; (c) a representative bright-field TEM image of an interface; top inset shows the dark-field image of the region while the bottom inset shows the HRTEM image of different orientation of the lattice fringes at the interface; (d) electron diffraction spots with their indexing corresponding to the pattern shown in (b); red and blue colors indicate the  $\text{BiFeO}_3$  and  $\text{Bi}_2\text{Fe}_4\text{O}_9$  phases, respectively.

In Fig. 3, we show the (a) full hysteresis loops corresponding to the data shown in Fig. 1a of the main paper and (b) the full hysteresis loops corresponding to the data shown in Fig. 1b of the paper. Likewise in Fig. 4, we show the full hysteresis loops corresponding to the Figs. 1c and 1d of the paper. The full hysteresis loops measured under zero-field cooled condition for determining

TABLE I. Structural details of the phases in the nanocomposite from FullProf refinement of x-ray diffraction data.

| Phase                                                    | Lattice Parameters<br>(Å)                    | Ions | Wyckoff Positions | x         | y          | z          | Bonds Length<br>(Å) | Bonds   | Angle<br>(°) | Crystallite Size | Volume Fraction |
|----------------------------------------------------------|----------------------------------------------|------|-------------------|-----------|------------|------------|---------------------|---------|--------------|------------------|-----------------|
| BiFeO <sub>3</sub><br>(R3c)                              | a = 5.579(5)<br>c = 13.863(7)                | Bi   | 6a                | 0.0       | 0.0        | 0.0        | Bi-O 2.282(3)       | Fe-O-Fe | 152.19(7)    | 111.9            | 93.89           |
|                                                          |                                              | Fe   | 6a                | 0.0       | 0.0        | 0.2251(5)  | Bi-O 2.499(5)       | O-Bi-O  | 72.36(4)     |                  |                 |
|                                                          |                                              | O    | 18b               | 0.4392(3) | 0.01530(6) | -0.0482(4) | Fe-O 1.918(5)       |         |              |                  |                 |
|                                                          |                                              |      |                   |           |            |            | Fe-O 2.165(3)       |         |              |                  |                 |
| Bi <sub>2</sub> Fe <sub>4</sub> O <sub>9</sub><br>(Pbam) | a = 7.976(6)<br>b = 8.479(9)<br>c = 6.008(3) | Bi   | 4g                | 0.1624(3) | 0.1597(5)  | 0.0        | Bi-O 2.461(3)       | Fe-O-Fe | 129.79(5)    | 19.3             | 6.11            |
|                                                          |                                              | Fe1  | 4f                | 0.5       | 0.0        | 0.2669(3)  | Bi-O 2.295(2)       | O-Bi-O  | 65.72(3)     |                  |                 |
|                                                          |                                              | Fe2  | 8i                | 0.3682(5) | 0.3356(7)  | 0.5        | Bi-O 2.438(3)       |         |              |                  |                 |
|                                                          |                                              | O1   | 2b                | 0.0       | 0.0        | 0.5        | Fe-O 2.092(4)       |         |              |                  |                 |
|                                                          |                                              | O2   | 8i                | 0.3722(7) | 0.2147(6)  | 0.2425(6)  | Fe-O 1.545(7)       |         |              |                  |                 |
|                                                          |                                              | O3   | 4f                | 0.1337(4) | 0.4039(2)  | 0.5        | Fe-O 2.016(4)       |         |              |                  |                 |
|                                                          |                                              | O4   | 4g                | 0.1534(6) | 0.4303(6)  | 0.0        |                     |         |              |                  |                 |
|                                                          |                                              |      |                   |           |            |            |                     |         |              |                  |                 |

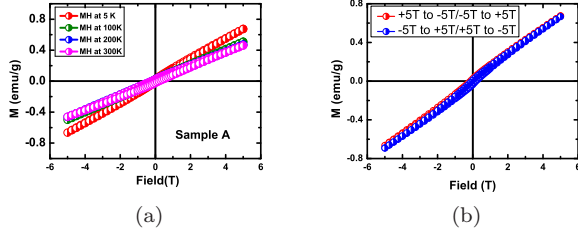

FIG. 3. (color online) (a) The complete form of the hysteresis loops measured under zero-field cooled condition to determine the spontaneous exchange bias (SEB) in sample-A; the portion near the origin is blown up in Fig. 1a of the main text to highlight the extent of SEB; (b) the complete form of the hysteresis loop measured at 5 K under zero-field cooled condition following two different paths - starting with +5T and -5T to show the difference in the extent of SEB ( $\Delta H_E$ ) depending on the sign of the starting field; a portion near the origin is blown up in Fig. 1b of the main text to highlight the asymmetry in SEB at 5 K.

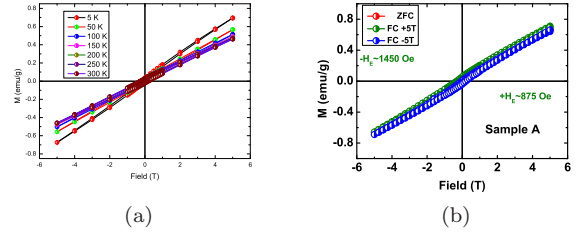

FIG. 4. (color online) (a) The complete form of the hysteresis loops measured following field cooling under a field of +5T to determine the conventional exchange bias (CEB) in sample-A; the portion near the origin is blown up in Fig. 1c of the main text; (b) the complete form of the hysteresis loops, measured at 5 K following field cooling under +5T, using two different tracing paths - one with +5T as the starting field and another with -5T as the starting field. It shows the difference in the extent of CEB ( $\Delta H_E$ ) depending on the sign of the starting field; a portion near the origin is blown up in Fig. 1b of the main text to highlight the asymmetry in CEB at 5 K.

the SEB in sample-B are shown in Fig. 5a. The asymmetry in the SEB at 5 K in sample-B depending on the sign of the starting field and the path followed in tracing the loop is shown in Fig. 5b. The Fig. 5c shows the variation in SEB and coercivity  $H_C$  with temperature for the sample-B. In Fig. 6 of this document, we show the hysteresis loops measured following field cooling under +5T. In Fig. 7a, we show the hysteresis loops measured following zero-field cooling for sample-C. Fig. 7b shows the blown-up portion of the loops around the origin.

We have also verified the presence of superspin glass moments in sample-B below the blocking temperature  $T_B \sim 60$  K. In Fig. 8, we show the characteristic dip at  $T_w \sim 21$  K in differential magnetization versus temperature plot signifying the memory effect. This has been observed

in sample-A as well as discussed in the main text of the paper. As expected, for sample-B also no signature of this memory effect could be seen at above  $T_B$ .

Finally, we discuss the importance of demagnetization prior to the measurement of the magnetic properties. The sample has been demagnetized by the following protocol: application of an oscillating field with varying amplitude; the amplitude reduces from maximum to zero. For example, for a demagnetizing field 1000 Oe, the amplitude is brought down to zero in the following sequence: (+1000)-(-900)-(+800)-(-700)...(+50)-(-40)...(+5)-(-4)-(+3)-(-2)-(+1)-(0). In Fig. 9, we show the difference in the ZFC, FC, and remanent magnetization for sample-A measured before and after demagnetization.

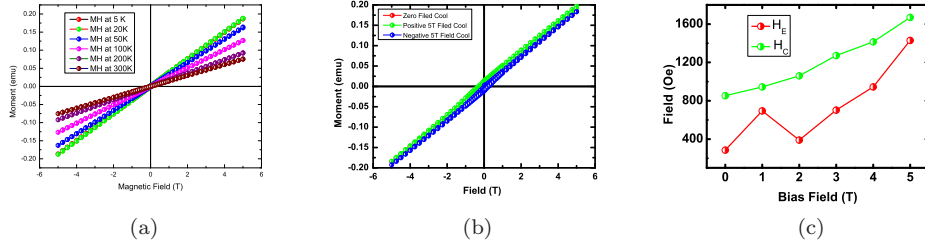

FIG. 5. (color online) (a) The hysteresis loops measured at different temperatures under zero-field cooled condition to determine the SEB in sample-B; (b) the hysteresis loops measured at 5 K via two different paths - with +5T or -5T as the starting field; (c) the temperature dependence of spontaneous exchange bias  $H_E$  and coercivity  $H_C$  in sample-B.

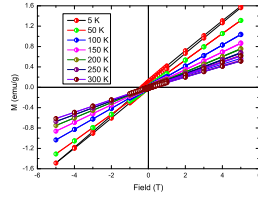

FIG. 6. (color online) The hysteresis loops measured at different temperatures following field cooling under +5T to determine the CEB in sample-B.

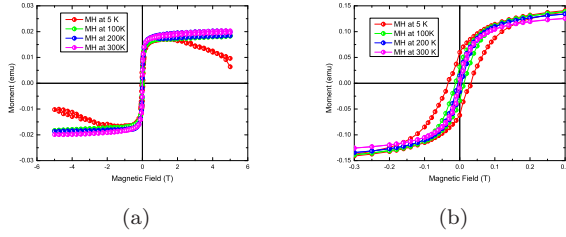

FIG. 7. (color online) (a) The hysteresis loops measured at different temperatures under zero-field cooled condition in sample-C; (b) portion of the loops near the origin is blown up.

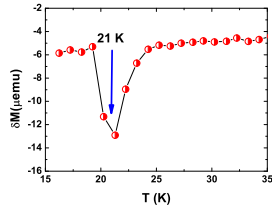

FIG. 8. (color online) The memory effect observed in sample-B at  $\sim 21$  K; no such effect has been observed at  $\sim 100$  K, i.e., above  $T_B$  ( $\sim 60$  K). This confirms the presence of superspin glass moments in sample-B as well below  $T_B$ .

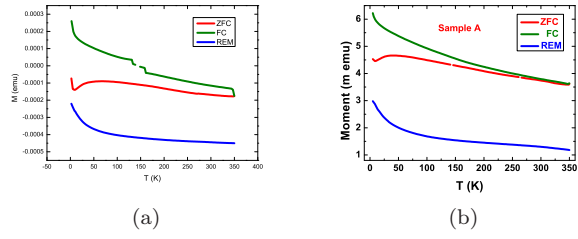

FIG. 9. (color online) The ZFC, FC, remanent magnetization measured in sample-A at (a) before and (b) after demagnetization.
